# Supplementary material for: Career Transitions and Trajectories: A Case Study in Computing
Source: arXiv:1805.06534 source file (2018-05-24)
Supplement: Supplementary file 1 [file 100_appendix.tex]

\ts{more data preprocessing info here}
